# Supplementary material for: Learning to Remember: A Synaptic Plasticity Driven Framework for Continual Learning
Source: arXiv:1904.03137 source file (2019-12-02)
Supplement: Supplementary file 1 [file appendix.tex]

\begin{comment}
\begin{table}[!h]
      
      \centering
      \scalebox{0.96}{
      \begin{tabular}[b]{lcccccc}
        \toprule 
        $\lambda$ & $2e^{-6}$ & $2e^{-1}$ & $0.75$ & $1$ & $2$ & $5$  \\
        \midrule
        $A_{5}(\%)$ & 98.35 & 98.10 & 97.22 &  96.91& 96.67& 88.70\\
        $Size$   & 364 &352 & 311& 286 & 261  &193\\\hline
      \end{tabular}}
    \caption{Sensitivity of parameter $\lambda_{RU}$ (MNIST benchmark).} %
    \label{tab:lambda_sens_}
\end{table}
\end{comment}

\section{DGM Losses.}
\label{app:losses}
The generator optimization problem at learning time of task $t$ can be formulated as minimizing $\mathcal{L_G}$, which is given by:
\begin{equation}
\min_{\theta_G} \mathcal{L_G} =\min_{\theta_G} (\mathcal{L}_s^G - \mathcal{L}_c^G+ \lambda_{RU} R^t),
\end{equation}
with individual components given as:
\begin{align} 
& \mathcal{L}_s^G = - \mathbb{E}_{z \sim p_z, y \sim p_c^t}[L_{adv.}(G_{\theta^G}(M_t, z, y))],  \\      
& \mathcal{L}_c^G = \mathbb{E}_{z \sim p_z,y \sim p_c^t}[y  \log(L_{aux}(G_{\theta^G}(M_t,z,y )))],
\end{align}                                                                
where $\mathcal{L}_c^G$ is the cross entropy loss calculated for generated samples on the auxiliary output of the discriminator, $\mathcal{L}_s^G$ a the adversarial loss calculated on the $L_{adv}.$  output layer of the $D$, $R^t$ is the regularization term presented in Eq.\ref{eq:reg}, and $\lambda_{RU}$ denotes the regularization weight meta-parameter. Further, $p_c^t=\mathcal{U}(1,|y^t|)$ is a uniform distribution over the labels of the task $t$, $p_z$ is the random noise distribution ($p_z \sim \mathcal{N}(0,1)$).

The discriminator is optimized  through minimizing $\mathcal{L_D}$, which can be formulated as:
\begin{align}
\min_{\theta_D} \mathcal{L_D}= \min_{\theta_D}(\mathcal{L}_s^D + \mathcal{L}_c^D+ \lambda_{GP}\mathcal{L}_{gp}^t).
\end{align}
The individual components are given as:
\begin{align}
 \mathcal{L}_s^D = - \mathbb{E}_{x_r \sim p_r^t} [L_{adv.}(x)] + \mathbb{E}_{x_f \sim p_g^t}[L_{adv.}(x_f)],
 \end{align}
\begin{multline}
\mathcal{L}_c^D = -   \mathbb{E}_{x_r,y \sim p_{r}^t(x,y)}[y \log L_{aux}(x_r)] - 
\\ \sum_{j=0}^{t-1} \mathbb{E}_{x_f,y^{\prime} \sim p_g^j(x,y) } [y^{\prime}  \log L_{aux}( x_f )],
\label{eq:L_c_D}
\end{multline}

where, $p_r^t$ is the distribution of real data for task $t$, $p_g^t$ is the distribution modeled by the generator ($x_f \sim p_g^t$ is equivalent to $x_f=G_{\theta^G}(M_t,z,y), z \sim p_z, y \sim p_c^t$). Hereby, the last term in Eq.\ref{eq:L_c_D} is the replay loss for previously seen categories,
$\mathcal{L}_{gp}^t$ is the gradient penalty of WGAN-GP \cite{gulrajani2017improved} formulated as:
\begin{equation}  
\mathcal{L}_{gp}^t = \mathbb{E}_{x_f \sim p_g^t}[(|| \nabla_{x_f} L_{adv.}(x_f)||_2-1)^2 ].
\end{equation}

\section{No-expansion Strategy}
\label{app:expansion} 
The importance of network capacity expansion can be demonstrated by assessing a model without the said expansion component. Fig.\ref{fig:no_size_exp} illustrates the dynamics of classification accuracy for the classes seen so-far for DGM with and without the network expansion component. It can be observed, that after a number of incoming tasks, the classification performance of the system drops significantly when the network expansion component is omitted (dashed lines). This illustrates that $G$ is not able to effectively memorize new information without an increase in capacity. In contrast, dynamic capacity expansion leads to stable and high classification accuracy (solid lines).
\begin{figure}[H]
  \includegraphics[width=\linewidth]{images/acc_axp_vs_no_axp.pdf}    
  \caption{Effect of the expansion component of DGM on MNIST.%
  }%
  \label{fig:no_size_exp}
\end{figure}

\section{Mask Learning DGMw}  
\label{app:DGMw_plast}                         
Fig.~\ref{fig:maskvals_DGMw} plots the plasticity learning behaviour of DGMw. One can observe, that the number of mask elements changing their value is constantly decreasing as the mask converges to the optimal parameter allocation. The overall layer occupation (bold blue line) is slowly increasing as the optimal number of parameters required for the task $t$ is learned. As detailed in Chapter \ref{sec:method}, the parameter $s$ of DGMw is annealed locally (over the number of batches) and globally (over the course of epochs). The local annealing component of DGMw permits 	masks learning during the entire training time of a tsk $t$. %
The mask learning behaviour of DGMw is different from the one of DGMa, since DGMa only features global annealing of $s$.

\begin{figure}[!h]  
\includegraphics[width=\linewidth]{images/masks_DGMw.pdf} 
    \caption{Trajectories of mask value change for a layer of G and task $t$ for DGMw. Solid blue line corresponds to layer occupation.}%
    \label{fig:maskvals_DGMw}%
\end{figure}

\begin{comment}
\section{Dynamic accuracy of DGM for different ratios $r$ vs. joint training upper bound.}
\label{sec:detailed_r}

\begin{figure*}[!h] 
  \includegraphics[width=\linewidth]{images/accs_top_5_diff_r.pdf} 
  \caption{Average top-5 performance of DGMw for different values of the ratio $r$ (ratio of real samples over the total number of replayed samples per each class)}%
  \label{fig:acc_r_}
\end{figure*}
\end{comment}

\section{ImageNet-50 Benchmark.} 
We use an identical generator structure to the one used for the CIFAR-10 benchmark - a ResNet like architecture proposed by~\cite{radford2015unsupervised}. The discriminator is replaced by a ResNet-18 discriminator. For the ImageNet-50 we use classes of iILSVRC-2012\cite{krizhevsky2012imagenet} dataset listed in Tab.\ref{tab:classes_Im_net}.
\begin{table}[!h]
      \small
      \centering
      \scalebox{0.96}{
      \begin{tabular}[b]{lc}
        \toprule 
        Task & Class indicies   \\
        \midrule
        Task 1 & [1, 15, 29, 45, 59, 65, 81, 89, 90, 99] \\
        Task 2   & [101, 115, 129, 145, 159, 165, 181, 189, 190, 199]  \\
        Task 3   & [201, 215, 229, 245, 259, 265, 281, 289, 290, 299]  \\
        Task 4   & [301, 315, 329, 345, 359, 365, 381, 389, 390, 399]  \\
        Task 5   & [401, 415, 329, 445, 459, 465, 481, 489, 490, 499]  \\        \hline
      \end{tabular}}
    \caption{ImageNet classes used for ImageNet-50 benchmark.} %
    \label{tab:classes_Im_net}
\end{table}

\begin{figure*}[!h]
     \centering              
     \subfloat[After 5 classes -   $A_5$]{{\includegraphics[width=0.23\linewidth]{images/conf_matrix_A_5.pdf}}}
    \subfloat[After 10 classes - $A_{10}$]{{\includegraphics[width=0.23\linewidth]{images/conf_matrix_A_10.pdf}}}
     \subfloat[Forgetting]{{\includegraphics[width=0.23\linewidth]{images/conf_forgetting.pdf}}}
    \caption{Confusion matrix for DGM's classification of SVHN samples after 5 (a) and after 10 classes (b); as well as for the case when no replay is performed (c) resulting in catastrophic forgetting. }%
    \label{fig:conf_matr}%
\end{figure*}

\section{Confusion analysis}
\label{app:conf_annalysis}    
We analyse the confusion matrices for the classification of the SVHN dataset after learning 5 classes - 
Fig.\ref{fig:conf_matr}(a), and 10 class - Fig.\ref{fig:conf_matr}(b). Here, the class predictions are mostly biased towards the currently learned class for which the real samples are available. This demonstrates that more expressive real samples tend to confuse the classifier towards the currently learned classes. In other words, the disparity in the expressive power of the training samples of different classes causes confusion that results in a performance drop. Fig.\ref{fig:conf_matr}(c) shows the confusion matrix for an incrementally trained model for which no measures against catastrophic forgetting were undertaken. One can observe, that the effect of classification bias towards currently learned class is exactly what constitutes catastrophic forgetting. It can be concluded, that the amount of forgetting in the task solver of DGM depends on the quality of the generated samples and the amount of mismatch in the expressive power of the generated and real data.

\section{Dynamics of FID score on ImageNet-50}
\label{app:fid_dynamics}
Per task dynamics of FID score for ImageNet-50 benchmark is presented in Fig.\ref{fig:fid_acc}. Here, higher values of FID correspond to worse perceptual quality of generated images and lower diversity. Note, for the calculation of FID of a given task $t$, we use the distribution of real images of this particular task as the ground truth.
\begin{figure}[h]%
    \centering                                                       
\includegraphics[width=\linewidth]{images/FID-imnet.pdf}
\caption{FID score dynamics of the ImageNet-50 benchmark.}%
   \label{fig:fid_acc}%
\end{figure}
\section{Growth pattern saturation}
\label{app:log_growth}

The non-saturating (yet sub-linear) growth pattern of the network presented in Fig.\ref{fig:masksizes} can be mainly attributed to the fact, that with the growing number of learned tasks, it becomes increasingly harder for the network to find those units, that can effectively contribute to the learning of a new task - i.e. with a growing amount of knowledge, selecting relevant knowledge becomes harder. This can be partially remedied by continuously increasing the learning time for each task, resulting growth pattern is shown in Fig. \ref{fig:maskvals_log}(a). Here, a network with a slightly higher initialization size then in Fig. ~\ref{fig:masksizes}(a) (best performing pattern) demonstrates a saturating growth pattern (decreasing slope), while the number of epochs for each task is increased gradually. %

\begin{figure}[!h]%
    \centering                   
    \subfloat[Saturating network growth.] {{\includegraphics[width=\linewidth]{images/network_growing_log.pdf}}}
    \\
    \subfloat[Network growth per layer with  saturating pattern]{{\includegraphics[width=\linewidth]{images/network_growing_log_per_layer_log.pdf}}}  

\caption{Growth pattern with graduelly increasing learning time in (a) togather with per layer growth pattern presented in (b).} %
    \label{fig:maskvals_log}%
\end{figure}

\begin{comment}
\section{Samples generated by DGMw after incremental training on different datasets.}
Samples generated after incremental training on 5 tasks of ImageNet-50 benchmark are shown in Fig.\ref{fig:samples_imnet_1_3} and \ref{fig:samples_imnet_4_5}. Samples generaated after incremental training on 10-tasks (each containing 1 class) of CIFAR-10 benchmark are presented in Fig.\ref{fig:samples_CIFAR}.

\label{sec:gen_imagenet}
\begin{figure*}[!h]  
    \centering
  \includegraphics[width=0.8\linewidth]{images/Samples_ImageNet_1_3.png}     
  \caption{Samples of task 1-3 (from left to right) generated after learning the 5-th task of the ImageNet-50 benchmark.}%
  \label{fig:samples_imnet_1_3}
\end{figure*}

\begin{figure*}[!h]  
    \centering
  \includegraphics[width=0.8\linewidth]{images/Samples_ImageNet_4_5.png} 
  \caption{Samples of task 4-5 (from left to right) generated after learning the 5-th task of the ImageNet-50 benchmark.}%
  \label{fig:samples_imnet_4_5}
\end{figure*}
 \newpage
\label{sec:gen_cifar_svhn}
\begin{figure*}[!h]  
    \centering
  \includegraphics[width=0.6\linewidth]{images/CIFAR_Samples_2.png}     
  \caption{Samples generated by DGMw after incremental training on 10-classes of CIFAR-10 benchmark }%
  \label{fig:samples_CIFAR}
\end{figure*}

\end{comment}
